# Supplementary material for: 3D unknown view tomography via rotation invariants
Source: arXiv:2003.10107 source file (2020-03-23)
Supplement: Supplementary file 1 [file appendix.tex]

\section{Appendix}
\label{app:features}
Let use rewrite the definition of $\mu(r)$ as,
\begin{align}
\label{eq:radial_meas}
    \mu(r) &= \mathbb{E}_{\theta} \left \{ \widehat{\mathcal{P}_{\theta} V}(r) \right \} \nonumber \\ &= \sum\limits_{k=1}^{K} \alpha_k \mathbb{E}_{\theta} \left \{ \exp \left( {-2j \pi r(x_k \cos \theta  +y_k \sin \theta)} \right) \right \} \nonumber \\ 
    & = \sum\limits_{k=1}^{K} \alpha_k \mathbb{E}_{\theta} \{\exp \left(-2j \pi r r_k \cos (\theta-\varphi_k) \right) \} \\ \nonumber
    & \stackrel{(a)}{=} \sum\limits_{k=1}^{K} \alpha_i \frac{1}{2 \pi} \int\limits_{-\pi}^{\pi} \exp (-2 j \pi r r_k \cos (\theta-\varphi_k)) d \theta \\ \nonumber
    & \stackrel{(b)}{=} \sum\limits_{k=1}^{K} \alpha_k J_{0}(2 \pi r r_k)
\end{align}
where (a) is due to the uniform assumption on projection directions, i.e. $\theta$. Also, (b) is obtained due to the periodicity of $\cos $ function alongside the definition of the Bessel function of the first kind and zeroth order \textcolor{blue}{cite a reference here}.

Similarly, for the second order feature we have,
\begin{align}
    C(r) &= \mathbb{E}_{\theta} \{\vert \widehat{\mathcal{P}_{\theta} V}(r) \vert^2 \} \label{eq:cov} \\
\begin{split}
     = \mathbb{E}_{\theta} \left\{ & \left( \sum\limits_{n=1}^{K} \alpha_n \exp (-2j \pi r r_n \cos (\theta-\varphi_n)) \right). \right. \\
    & \left. \left(\sum\limits_{m=1}^{K} \alpha_m \exp(2j \pi r r_m \cos (\theta-\varphi_m)) \right) \vphantom{\int_1^2} \right\} \nonumber \\
    % & = \mathbb{E}_{\omega} \left\{ \left(\sum\limits_{n=1}^{K} \sum\limits_{m=1}^{K} \alpha_n \alpha_m e^{-j r r_n \cos (\phi_{\omega}-\phi_n)}  e^{+j r r_m \cos (\phi_{\omega}-\phi_m)} \right)  \right\} \\ \nonumber
    \end{split}
    % \begin{split}
    % \left( \int_1^2 ba ba \mathrm da \right. \\
    % \left. ba ba ba \vphantom{\int_1^2} \right)
    % \end{split}
    \end{align}
    \begin{align}
    &= \sum\limits_{n=1}^{K} \sum\limits_{m=1}^{K} \alpha_n \alpha_m \mathbb{E}_{\theta} \left\{ e^{-2j \pi r (\cos \theta \Delta x_{n,m} + \sin \theta \Delta y_{n,m})} \right\} \nonumber
    \end{align}
where $\Delta x_{n,m} = x_n - x_m$ and $\Delta y_{n,m} = y_n - y_m$. Next,
\begin{align}
    & \stackrel{=}{(a)} \sum\limits_{n=1}^{K} \sum\limits_{m=1}^{K} \alpha_n \alpha_m \mathbb{E}_{\theta} \{e^{-2j \pi r d_{n,m} (\frac{\Delta x_{n,m}}{d_{n,m}} \cos \theta +  \frac{\Delta y_{m,n}}{d_{n,m}} \sin \theta)} \} \nonumber \\
    & = \sum\limits_{n=1}^{K} \sum\limits_{m=1}^{K} \alpha_n \alpha_m \mathbb{E}_{\theta} \{\exp \left(-2j \pi r d_{n,m} \cos (\theta - {\varphi}_{n,m}) \right) \} \nonumber \\
    & = \sum\limits_{n=1}^{K} \sum\limits_{m=1}^{K} \alpha_n \alpha_m \int\limits_{- \pi}^{\pi} \frac{1}{2 \pi} e^{-2j \pi r d_{m,n} \cos (\theta - {\varphi}_{n,m})} d \theta \nonumber \\
    & = \sum\limits_{n=1}^{K} \sum\limits_{m=1}^{K} \alpha_n \alpha_m J_{0}(2 \pi r d_{m,n}). \label{eq:D}
\end{align}
Note that in (a), $\varphi_{n,m}$ correspond to the angle of $(x_n-x_m,y_n-y_m)$ with the $x$-axis in the Cartesian coordinate system.
